# Supplementary material for: Seaweed-7B: Cost-Effective Training of Video Generation Foundation Model
Source: arXiv:2504.08685 source file (2025-05-05)
Supplement: Supplementary file 1 [file 9_appendix.tex]

%\section*{Appendix}
%\subsection{VAE implementation details}
% Specifically, the 3D convolution blocks inside both the encoder and the decoder are causal along the temporal dimension. To ensure complete causality, we also change the group normalizations to 2D to avoid temporal leakage. This design allow us to process an arbitrarily long video by chunks along the temporal dimension. When processing the current chunk, every causal convolution layer stores a small slice of the tailing pixels. This slice of pixels are reloaded as the leading paddings when processing the next chunk. As a result, the full receptive field is preserved and the output results are fully equivalent to processing the entire clip without chunking.

% \todo{add VAE details}

% \paragraph{VAE architecture}

% \paragraph{Training hyper-parameters}
